# Supplementary material for: The Best of Both Worlds: On the Dilemma of Out-of-distribution Detection
Source: arXiv:2410.11576 source file (2024-10-12)
Supplement: Supplementary file 1 [file table1.tex]

\begin{table}[htbp]
\begin{center}
% \begin{spacing}{1.35}   
%\small
\caption{OOD generalization performance comparison. We report the mean accuracy in five random runs on post-hoc methods and three random runs on other methods on covariate-shifted test set under various types of noise. The \textbf{best} and \underline{second best} are highlighted in bold or underlined.}
\label{tab:diverse-noise-types}
\center
\resizebox{1.0\textwidth}{!}{
\begin{tabular}{ccccccc} % Modified column declaration
\toprule                                              
$\mathcal{P}^{\rm in}/\mathcal{P}^{\rm aux}$ & Type  &Method & \text{GaussianNoise. $\uparrow$} & \text{SaltPepperNoise $\uparrow$}& \text{NormalBlur $\uparrow$} & \text{MeanBlur $\uparrow$} \\ \midrule
\multirow{4}{*} {\shortstack{CIFAR-10\\ \\Only}} &\multirow{4}{*} {Post-hoc}         &MSP        &  $87.35$   &   $69.92$ & $69.76$ & $76.11$ \\ & &EBM (pretrain)     &  $87.35$   &   $69.92$ & $69.76$ & $76.11$  \\& &Maxlogits     &  $87.35$   &   $69.92$ & $69.76$ & $76.11$ \\ & &Mahalanobis     &  $87.35$   &   $69.92$ & $69.76$ & $76.11$   \\ \midrule \multirow{8}{*}{\shortstack{CIFAR10 \\ \\ImageNet-RC}} &\multirow{5}{*} {Training}
    
     &OE     &   $72.57$    & $54.56$                                                    &$67.61$    &$74.76$ \\&  
     &EBM (finetune)      &   $79.03$     &$53.42$                                                    &$66.49$ &$69.56$ \\&  
    
     &POEM      &   $78.89$     &$54.37$                                                    &$66.46$    & $68.21$   \\&  
    
    &DPN      &   $85.52$     &$56.14$                                                    &$66.77$    &$76.18$ \\&  
    
     &WOODS     &  $80.14$ &$56.31$                     &$69.00$  & $\textbf{78.00}$    \\ \cline{2-7} &\multirow{3}{*} {Two-target} &SCONE        &  $78.80$ &$55.37$                                                    &$68.11$    &$\underline{77.76}$ \\&
     &DUL (ours)     & \cellcolor{gray!20}$\textbf{88.01}$  &\cellcolor{gray!20}$\textbf{70.01}$                                                    &\cellcolor{gray!20}$\textbf{70.20}$    &\cellcolor{gray!20}$77.28$ \\&
     &DUL\textsuperscript{\dag} (ours)     & \cellcolor{gray!20}$\underline{87.53}$  &\cellcolor{gray!20}$\underline{69.04}$                                                    &\cellcolor{gray!20}$\underline{69.09}$    &\cellcolor{gray!20}$75.54$\\ \midrule \multirow{8}{*}{\shortstack{CIFAR10 \\ \\TIN-597}} &\multirow{5}{*} {Training}
    
    &OE       &   $80.51$    &$66.73$                                                    &$64.65$    & $72.67$                           \\& 
    
     &EBM (finetune)       &   $83.67$     &$61.81$                                                    &$67.08$    &$74.93$                             \\&
    
     &POEM        &  $83.17$ &$61.01$                                                    &$\textbf{70.48}$    &$76.48$                  \\& &DPN      &  $79.23$ &$63.19$                                                    &$66.24$     & $68.64$ \\& &WOODS     &  $83.12$ &$68.42$                                                    &$66.80$    & $74.30$ \\ \cline{2-7} &\multirow{3}{*} {Two-target} &SCONE      &  $84.68$ &$67.74$                 &$66.23$     & $75.61$                         \\&
     &DUL (ours)      & \cellcolor{gray!20}$\underline{87.93}$  &\cellcolor{gray!20}$\underline{71.25}$                                                    &\cellcolor{gray!20}$\underline{70.03}$    &\cellcolor{gray!20}$\underline{77.43}$   \\&
     &DUL\textsuperscript{\dag} (ours)      & \cellcolor{gray!20}$\textbf{88.10}$  &\cellcolor{gray!20}$\textbf{71.43}$                          &\cellcolor{gray!20}$69.93$    & \cellcolor{gray!20}$\textbf{77.53}$    \\ \midrule
\multirow{4}{*} {\shortstack{CIFAR-100\\ \\Only}} &\multirow{4}{*} {Post-hoc}    &MSP     &   $55.95$   &   $45.02$                                                 & $52.18$   & $58.78$  \\ & &EBM (pretrain)      &  $55.95$  &$45.02$                                                    &$52.18$    &$58.78$  \\& &Maxlogits     &  $55.95$  &$45.02$                                                    &$52.18$     &$58.78$\\ & &Mahalanobis    &  $55.95$  &$45.02$                                                    &$52.18$     &$58.78$   \\ \midrule \multirow{8}{*}{\shortstack{CIFAR100 \\ \\ImageNet-RC}} &\multirow{5}{*} {Training}
    
    &OE      &  $45.48$ &$41.24$                                                    &$51.10$    &$56.65$                              \\ & 
    
     &EBM (finetune)      &   $48.14$  &$41.05$                                                    &$51.09$    &$56.13$                              \\ & 
    
     &POEM      &  $42.18$ &$40.14$                                                    &$49.14$    &$54.61$                            \\& &DPN     &  $50.14$ &$41.33$                                                    &$51.39$  & $55.50$ \\ &&WOODS     &  $54.38$ &$43.85$                                                    &$\underline{52.13}$     & $\underline{58.86}$ \\ \cline{2-7} &\multirow{3}{*} {Two-target} &SCONE      &  $\textbf{56.73}$ &$\textbf{45.59}$                  &$\underline{52.13}$   & $58.78$                              \\& 
    
     &DUL (ours)      & \cellcolor{gray!20}$\underline{56.27}$ &\cellcolor{gray!20}$\underline{44.73}$                                                    &\cellcolor{gray!20}$\textbf{52.39}$   & \cellcolor{gray!20}${58.82}$   \\&
     &DUL\textsuperscript{\dag} (ours)      & \cellcolor{gray!20}$56.07$  &\cellcolor{gray!20}$44.42$                                                    &\cellcolor{gray!20}$51.97$     &\cellcolor{gray!20}$\textbf{59.17}$    \\ \midrule \multirow{8}{*}{\shortstack{CIFAR100 \\ \\TIN-597}} &\multirow{5}{*} {Training}
     &OE      &  $46.25$ &$43.67$                                                    &$50.44$    &$56.56$                             \\  &
    
     &EBM (finetune)      &   $50.00$  &$43.20$                                                    &$50.38$  & $\underline{57.48}$                             \\  &
    
     &POEM     &  $52.53$ &$42.76$                                                    &$51.20$    &$56.36$                         \\ &&DPN      &  $47.67$ &$43.45$         &$49.35$   & $55.34$ \\& &WOODS     &  $53.13$ &$44.41$                                                    &$51.47$     & $56.82$ \\ \cline{2-7} &\multirow{3}{*} {Two-target} &SCONE      &  $52.70$ &$44.42$                 &$\underline{51.63}$    &$56.73$                             \\ &
    
     &DUL (ours)      & \cellcolor{gray!20}$\underline{56.19}$ &\cellcolor{gray!20}$\textbf{45.38}$                                                    &\cellcolor{gray!20}$\textbf{51.77}$    &\cellcolor{gray!20}$\textbf{58.44}$    \\&
     &DUL\textsuperscript{\dag} (ours)      & \cellcolor{gray!20}$\textbf{56.22}$  &\cellcolor{gray!20}$\underline{44.89}$                                                    &\cellcolor{gray!20}$51.56$    & \cellcolor{gray!20}$57.35$  \\  
       \bottomrule
\end{tabular}}
\end{center}
\vskip -0.3in
\end{table}
