# Supplementary material for: The Best of Both Worlds: On the Dilemma of Out-of-distribution Detection
Source: arXiv:2410.11576 source file (2024-10-12)
Supplement: Supplementary file 3 [file table8.tex]

\begin{table}[htbp]
\begin{center}  
\caption{OOD generalization performance comparison. We report the mean classification accuracy in three random runs on covariate-shifted test set under various types of noise. The best and second best are highlighted in bold or underlined.}
\label{tab:diverse-noise-types}
\center
\resizebox{1.0\textwidth}{!}{

\begin{tabular}{ccccccc}
\toprule                                                          
$\mathcal{P}^{\rm in}/\mathcal{P}^{\rm aux}$ & Method &\text{GaussianNoise. $\uparrow$} & \text{SaltPepperNoise. $\uparrow$} & \text{NormalBlur $\uparrow$}& \text{GaussianBlur $\uparrow$}  &\text{MeanBlur $\uparrow$}  \\ \midrule \multirow{5}{*} {\shortstack{CIFAR-10\\ \\Only}}&\textit{Post-hoc}      &  &                                                    &  &    &                              \\
         
     &MSP        &  $87.35$   &  $69.92$                                                  &$69.47$  & $55.46$  & $73.35$                          \\ &Energy      &  $87.35$&  $69.92$                                                  & $69.47$ & $55.46$   &$73.35$                              \\&Maxlogits      &  $87.35$&  $69.92$                                                  & $69.47$ & $55.46$   &$73.35$                            \\&Mahalanobis      &  $86.14$&  $69.68$                                                  & $69.61$ & $55.72$   &$73.18$                                                             \\ \midrule \multirow{11}{*} {\shortstack{CIFAR-10\\ \\ImageNet-RC}}  
    
     &OE      &   $72.57$    & $54.56$                                                    &$67.61$  &$54.43$   &$74.76$                              \\  
    
     &Energy      &   $79.03$     &$53.42$                                                    &$66.49$  &$55.80$   &$69.56$                              \\  
    
     &POEM      &   $78.89$     &$54.37$                                                    &$66.46$  &$54.52$   & $68.21$               \\&DPN      &   $85.52$     &$56.14$                                                    &$66.77$  &$55.22$   &$76.18$  \\ &WOODS     &  $80.14$ &$56.31$                     &$69.00$  &$54.37$   & $78.00$                            \\ \cline{2-7} &\textit{Detection and generalization}      &   &                                                    &  &   &                             \\ &SCONE      &  $78.80$ &$55.37$                                                    &$68.11$  &$53.92$   &$77.76$                              \\
     &DUL (ours)      &  \cellcolor{gray!20}$88.01$  &\cellcolor{gray!20}$70.01$                                                    &\cellcolor{gray!20}$70.20$  &\cellcolor{gray!20}$56.29$   &\cellcolor{gray!20} $77.28$  \\
     &DUL\textsuperscript{\dag} (ours)      & \cellcolor{gray!20} $87.53$  &\cellcolor{gray!20}$69.04$                                                    &\cellcolor{gray!20}$69.09$  &\cellcolor{gray!20}$55.68$   & \cellcolor{gray!20}$75.54$                             \\ \midrule
\multirow{11}{*} {\shortstack{CIFAR-10\\ \\TIN-597}}         
     &\textit{Training}      &       &                                                    &  &   &                              \\
    
     &OE       &   $80.51$    &$66.73$                                                    &$64.65$  &$54.06$   & $72.67$                             \\  
    
     &Energy       &   $83.67$     &$61.81$                                                    &$67.08$  &$55.55$   &$74.93$                              \\  
    
     &POEM        &  $83.17$ &$61.01$                                                    &$70.48$  &$55.27$   &$76.48$                  \\ &DPN      &  $79.23$ &$63.19$                                                    &$66.24$  &$53.77$   & $68.64$ \\ &WOODS     &  $83.12$ &$68.42$                                                    &$66.80$  &$53.77$   & $74.30$
                          \\ \cline{2-7} &\textit{Two-target}      &   &                                                    &  &   &     \\&SCONE      &  $84.68$ &$67.74$                 &$66.23$  &$53.54$   & $75.61$                          \\
     &DUL (ours)      & \cellcolor{gray!20} $87.93$  &\cellcolor{gray!20}$71.25$                                                    &\cellcolor{gray!20}$70.03$  &\cellcolor{gray!20}$56.50$   &\cellcolor{gray!20}$77.43$   \\
     &DUL\textsuperscript{\dag} (ours)      & \cellcolor{gray!20} $88.10$  &\cellcolor{gray!20}$71.43$                          &\cellcolor{gray!20}$69.93$  &\cellcolor{gray!20}$55.87$   & \cellcolor{gray!20}$77.53$                               \\ \midrule
 \multirow{5}{*} { \shortstack{CIFAR-100\\ \\Only}}&\textit{OOD detection (Post-hoc)}      &  &                                                    &  &    &                              \\         
     &MSP    &   $55.95$   &   $45.02$                                                 & $52.18$ & $42.53$  & $58.78$                          \\ &Energy      &  $55.95$  &$45.02$                                                    &$52.18$  &$42.53$   &$58.78$                              \\
    
     &Maxlogits     &  $55.95$  &$45.02$                                                    &$52.18$  &$42.53$   &$58.78$                             \\&Mahalanobis    &  $55.84$  &$45.05$                                                    &$51.80$  &$42.21$   &$58.41$                             \\ \midrule \multirow{11}{*} { \shortstack{CIFAR-100\\ \\ImageNet-RC}}&\textit{OOD detection (training)}      &  &                                                    &  &    &                              \\  &OE      &  $45.48$ &$41.24$                                                    &$51.10$  &$42.00$   &$56.65$                              \\  
    
     &Energy      &   $48.14$  &$41.05$                                                    &$51.09$  &$41.96$   &$56.13$                              \\  
    
     &POEM      &  $42.18$ &$40.14$                                                    &$49.14$  &$40.57$   &$54.61$                            \\ &DPN     &  $50.14$ &$41.33$                                                    &$51.39$  &$42.01$   & $55.50$ \\ &WOODS     &  $54.38$ &$43.85$                                                    &$52.13$  &$42.68$   & $58.86$
                          \\ \cline{2-7} &\textit{Detection and generalization}      &  &                                                    &  &    &         \\&SCONE      &  $56.73$ &$45.59$                  &$52.13$  &$42.88$   & $58.78$                              \\ 
    
     &DUL (ours)      & \cellcolor{gray!20} $56.36$ &\cellcolor{gray!20}$44.73$                                                    &\cellcolor{gray!20}$52.39$  &\cellcolor{gray!20}$42.68$   &\cellcolor{gray!20} $58.82$   \\
     &DUL\textsuperscript{\dag} (ours)      & \cellcolor{gray!20} $55.41$  &\cellcolor{gray!20}$43.90$                                                    &\cellcolor{gray!20}$51.40$  &\cellcolor{gray!20}$41.89$   & \cellcolor{gray!20}$58.12$                              \\  \midrule
\multirow{11}{*} { \shortstack{CIFAR-100\\ \\TIN-597}}  &\textit{OOD detection (training)}      &  &                                                    &  &    &                              \\  &OE      &  $46.25$ &$43.67$                                                    &$50.44$  &$41.78$   &$56.56$                             \\  
    
     &Energy      &   $50.00$  &$43.20$                                                    &$50.38$  &$41.70$   & $57.48$                             \\  
    
     &POEM     &  $52.53$ &$42.76$                                                    &$51.20$  &$41.51$   &$56.36$                         \\ &DPN      &  $47.67$ &$43.45$         &$49.35$  &$41.04$   & $55.34$ \\ &WOODS     &  $53.13$ &$44.41$                                                    &$51.47$  &$42.11$   & $56.82$
                          \\ \cline{2-7} &\textit{Detection and generalization}      &  &                                                    &  &    &          \\&SCONE      &  $52.70$ &$44.42$                 &$51.63$  &$41.98$   &$56.73$                             \\ 
    
     &DUL (ours)      &\cellcolor{gray!20}  $56.19$ &\cellcolor{gray!20}$45.38$                                                    &\cellcolor{gray!20}$51.77$  &\cellcolor{gray!20}$42.63$   &\cellcolor{gray!20} $58.44$    \\
     &DUL\textsuperscript{\dag} (ours)      & \cellcolor{gray!20} $56.21$  &\cellcolor{gray!20}$44.89$                                                    &\cellcolor{gray!20}$51.56$  &\cellcolor{gray!20}$42.06$   &\cellcolor{gray!20} $57.35$                                           \\
       \bottomrule
\end{tabular}}
\end{center}
\end{table}
