# Supplementary material for: The Best of Both Worlds: On the Dilemma of Out-of-distribution Detection
Source: arXiv:2410.11576 source file (2024-10-12)
Supplement: Supplementary file 4 [file table7.tex]

\begin{table}[!htbp]
\vskip 0.15in
\begin{center}
% \begin{spacing}{1.35}   
%\small
\caption{OOD generalization performance comparison under diverse types of corruption. The superiority of our DUL is consistent across different types of corruption. The \textbf{best} and \underline{second best} are highlighted in bold or underlined.}
\label{tab:diverse-noise-types-imagenet}
\center
\resizebox{1.0\textwidth}{!}{
\setlength{\tabcolsep}{3.9mm}
\begin{tabular}{cccccc}
\toprule                                              
$\mathcal{P}^{\rm in}/\mathcal{P}^{\rm aux}$ & Type  &Method & \text{GaussianNoise. $\uparrow$} & \text{SaltPepperNoise $\uparrow$}& \text{MeanBlur $\uparrow$}  \\ \midrule
\multirow{8}{*} {\shortstack{ImageNet-200\\ \\ImageNet-800}} &\multirow{3}{*} {Post-hoc}         &MSP        &  $74.84$   &   $57.33$                                                  & $82.11$                           \\ & &Energy      &   $74.84$&   $57.33$                                                  &  $82.11$                               \\& &Maxlogits      &  $74.84$&  $57.33$                                                  & $82.11$                               \\ \cline{2-6} &\multirow{4}{*} {Training}
    
     &Entropy      &  ${74.75}$   &   $56.70$                                                  & $\underline{82.31}$                                                     \\&  
    
     &EBM (finetune)      &  $73.31$   &   $54.92$                                                  & $81.43$                                                             \\&  
    
     &DPN      &  $74.40$   &   $\underline{57.90}$                                                  & $82.20$                           \\&  
    
     &WOODS      &  $\underline{74.98}$   &   $57.65$                                                  & $82.17$                          \\ \cline{2-6} &\multirow{2}{*} {Two-target} &SCONE      &  $74.91$   &   $57.52$                                                  & $82.10$                                                      \\&
     &DUL (ours)      & \cellcolor{gray!20}$\textbf{75.59}$   & \cellcolor{gray!20}$\textbf{58.13}$                                                  &\cellcolor{gray!20}$\textbf{82.74}$                                                      \\  
       \bottomrule
\end{tabular}}
\end{center}
\end{table}
